# Supplementary material for: Quality-Diversity Actor-Critic: Learning High-Performing and Diverse Behaviors via Value and Successor Features Critics
Source: arXiv:2403.09930 source file (2024-06-03)
Supplement: Supplementary file 1 [file 4_implementation-details.tex]

\newpage
\section{Implementation Details}
\label{appendix:impl}

Distributional critic

Huber Loss: $L = \delta \left( \sqrt{1 + (\frac{x}{\delta})^2} - 1 \right)$

$\lambdaLagr$ does not depend on state.

Value lambda
